# Supplementary material for: A Contrast-Agnostic Method for Ultra-High Resolution Claustrum Segmentation
Source: arXiv:2411.15388 source file (2025-04-29)
Supplement: Supplementary file 1 [file SupplementaryMaterial.pdf]

# A Constrast-Agnostic Method for Ultra-High Resolution Claustrum Segmentation
# Supplementary materials

Chiara Mauri, Ryan Fritz, Jocelyn Mora, Benjamin Billot, Juan Eugenio Iglesias, Koen Van Leemput, Jean Augustinack, Douglas N Greve

### Supplementary Section 1: SmartInterpol

Supplementary Fig. 1.1 and Supplementary Fig. 1.2 show manual claustrum annotations on every 5th coronal slice, together with SmartInterpol-generated labels for the intermediate slices, and final manual corrections where applicable.

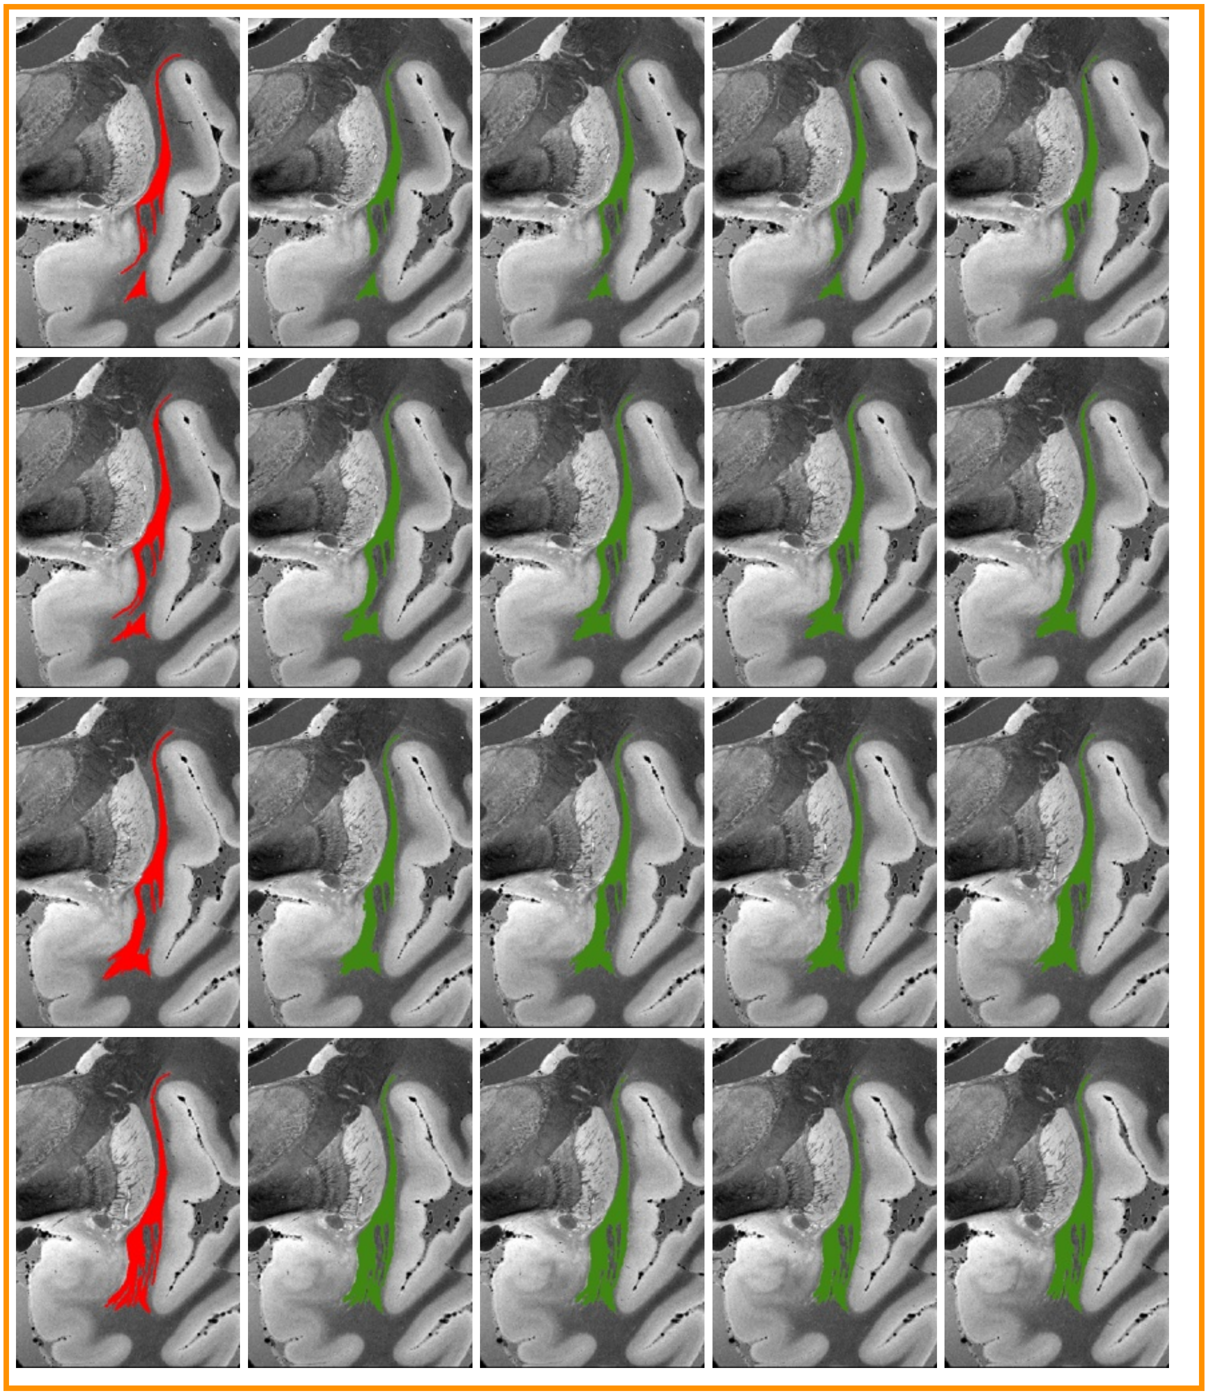

Supplementary Figure 1.1: Claustrum manual labels for case 14 in coronal views, slices 715 to 734. Red: Manual labels annotated every 5th slice. Green: Labels generated by SmartInterpol in the intermediate slices.

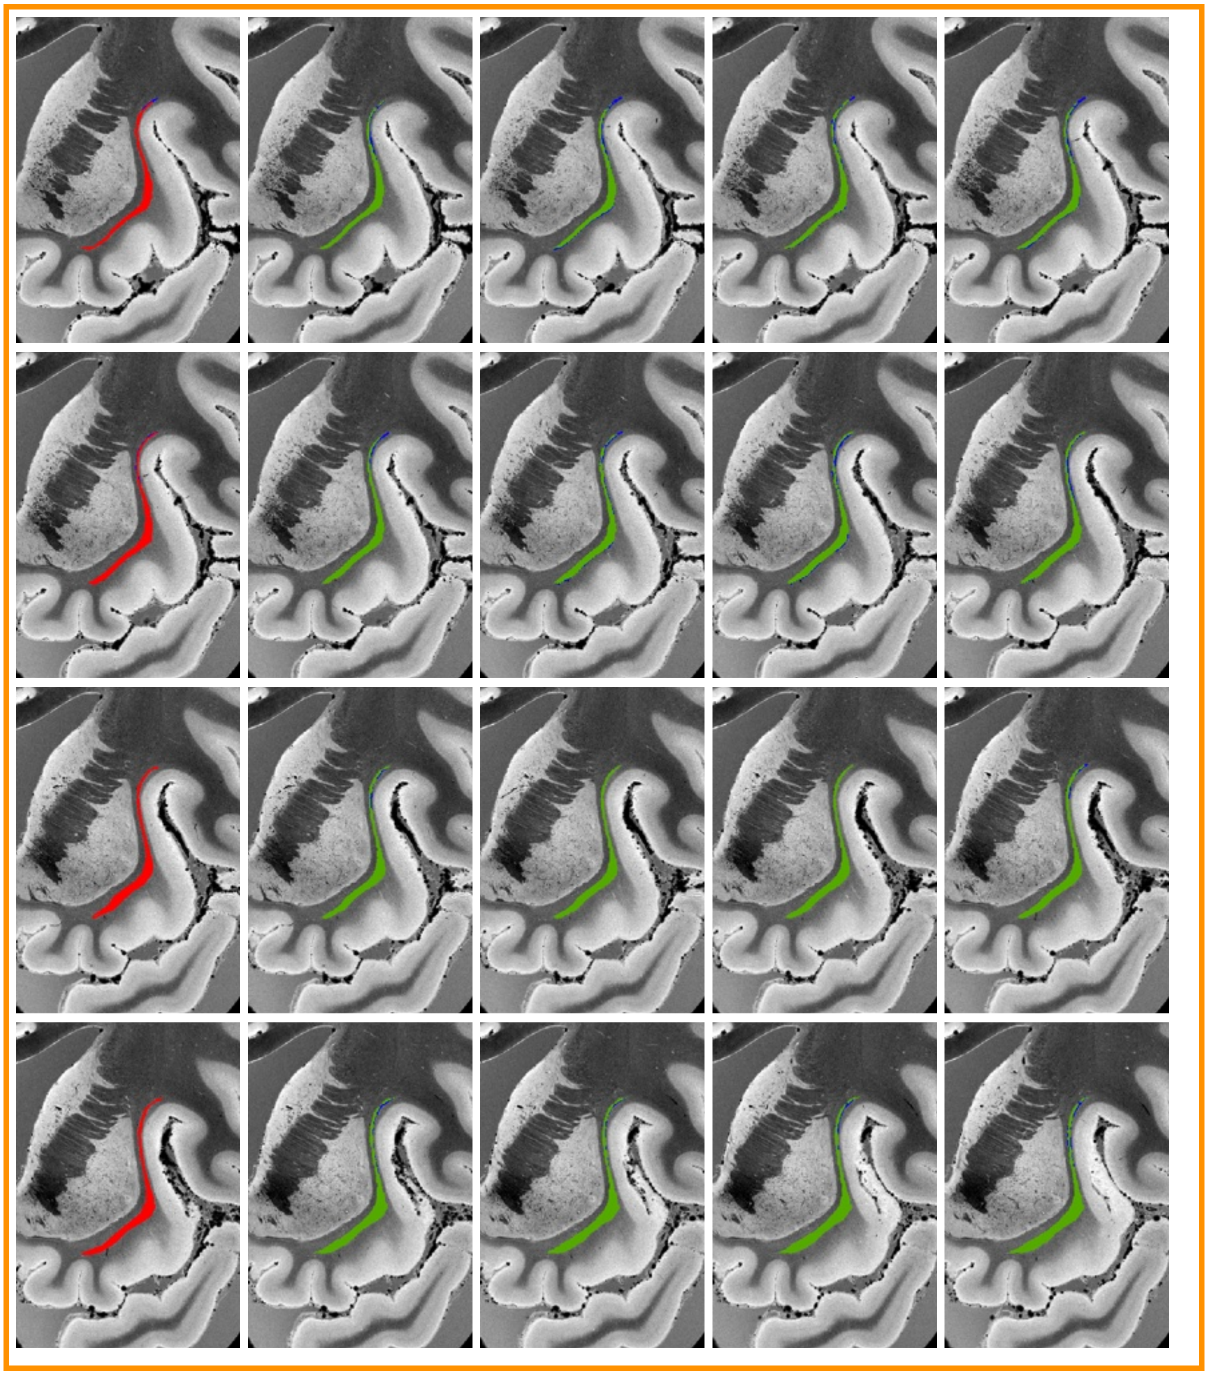

Supplementary Figure 1.2: Claustrum manual labels for case 14 in coronal views, slices 615 to 634. Red: Manual labels annotated every 5th slice. Green: Labels generated by SmartInterpol in the intermediate slices. Blue: Manual corrections made after applying SmartInterpol.

### Supplementary Section 2: Synthetic intensity images

Supplementary Fig. 2.1 shows coronal views of augmented labels and their corresponding synthetic intensity images generated during training.

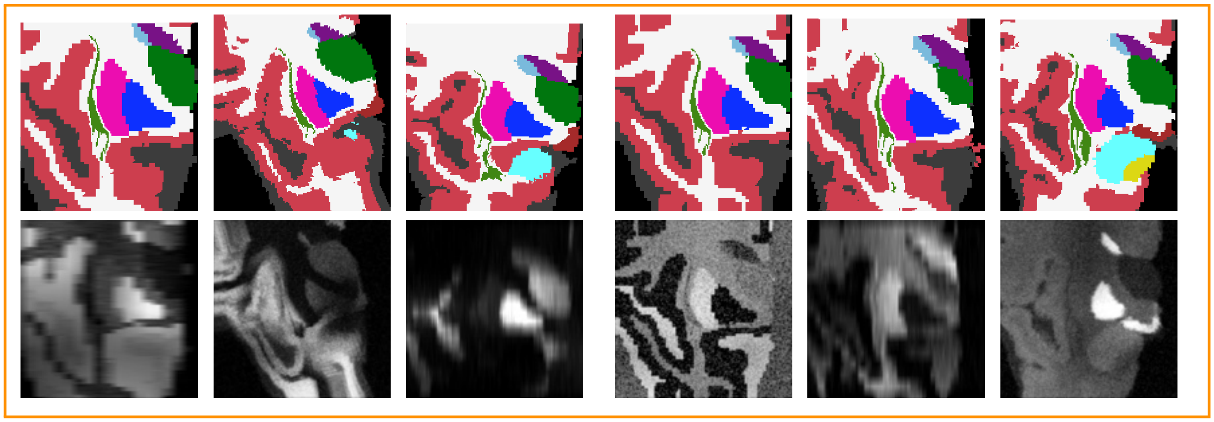

Supplementary Figure 2.1: Top: Example of augmented labels derived from the label shown in Fig. 5 (case 14, coronal view, slice number 247). Bottom: Corresponding synthetic images generated with random contrast.

### Supplementary Section 3: Claustrum probabilistic atlas

Supplementary Fig. 3.1, Supplementary Fig. 3.2, and Supplementary Fig. 3.3 show coronal slices of the probabilistic atlas for right claustrum in MNI152 space, from posterior to anterior. Supplementary Fig. 3.4 displays the 3D rendering of the atlas thresholded at 0.05 for visualization.

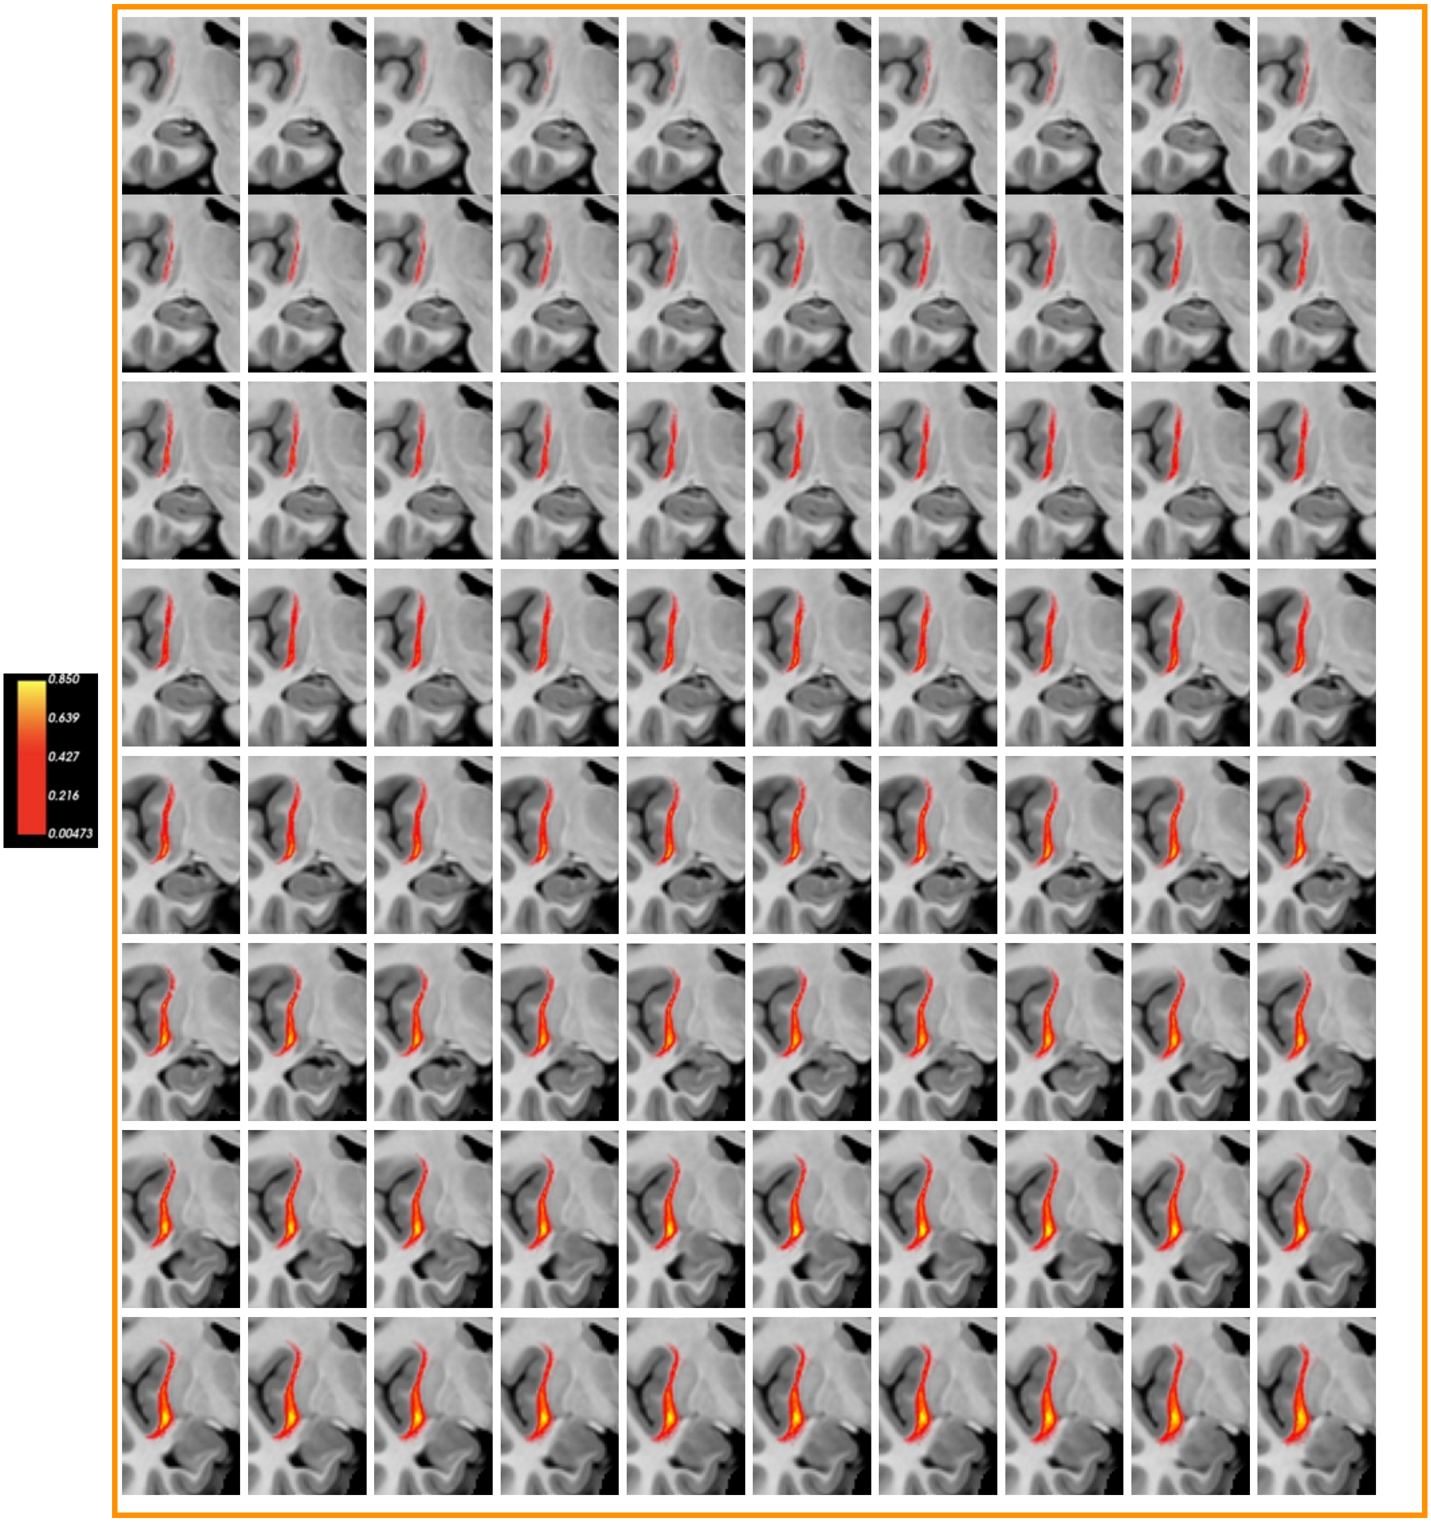


Supplementary Figure 3.1: Coronal slices of the claustrum probabilistic atlas in MNI space, for the right hemisphere (slice numbers: 70 to 149).

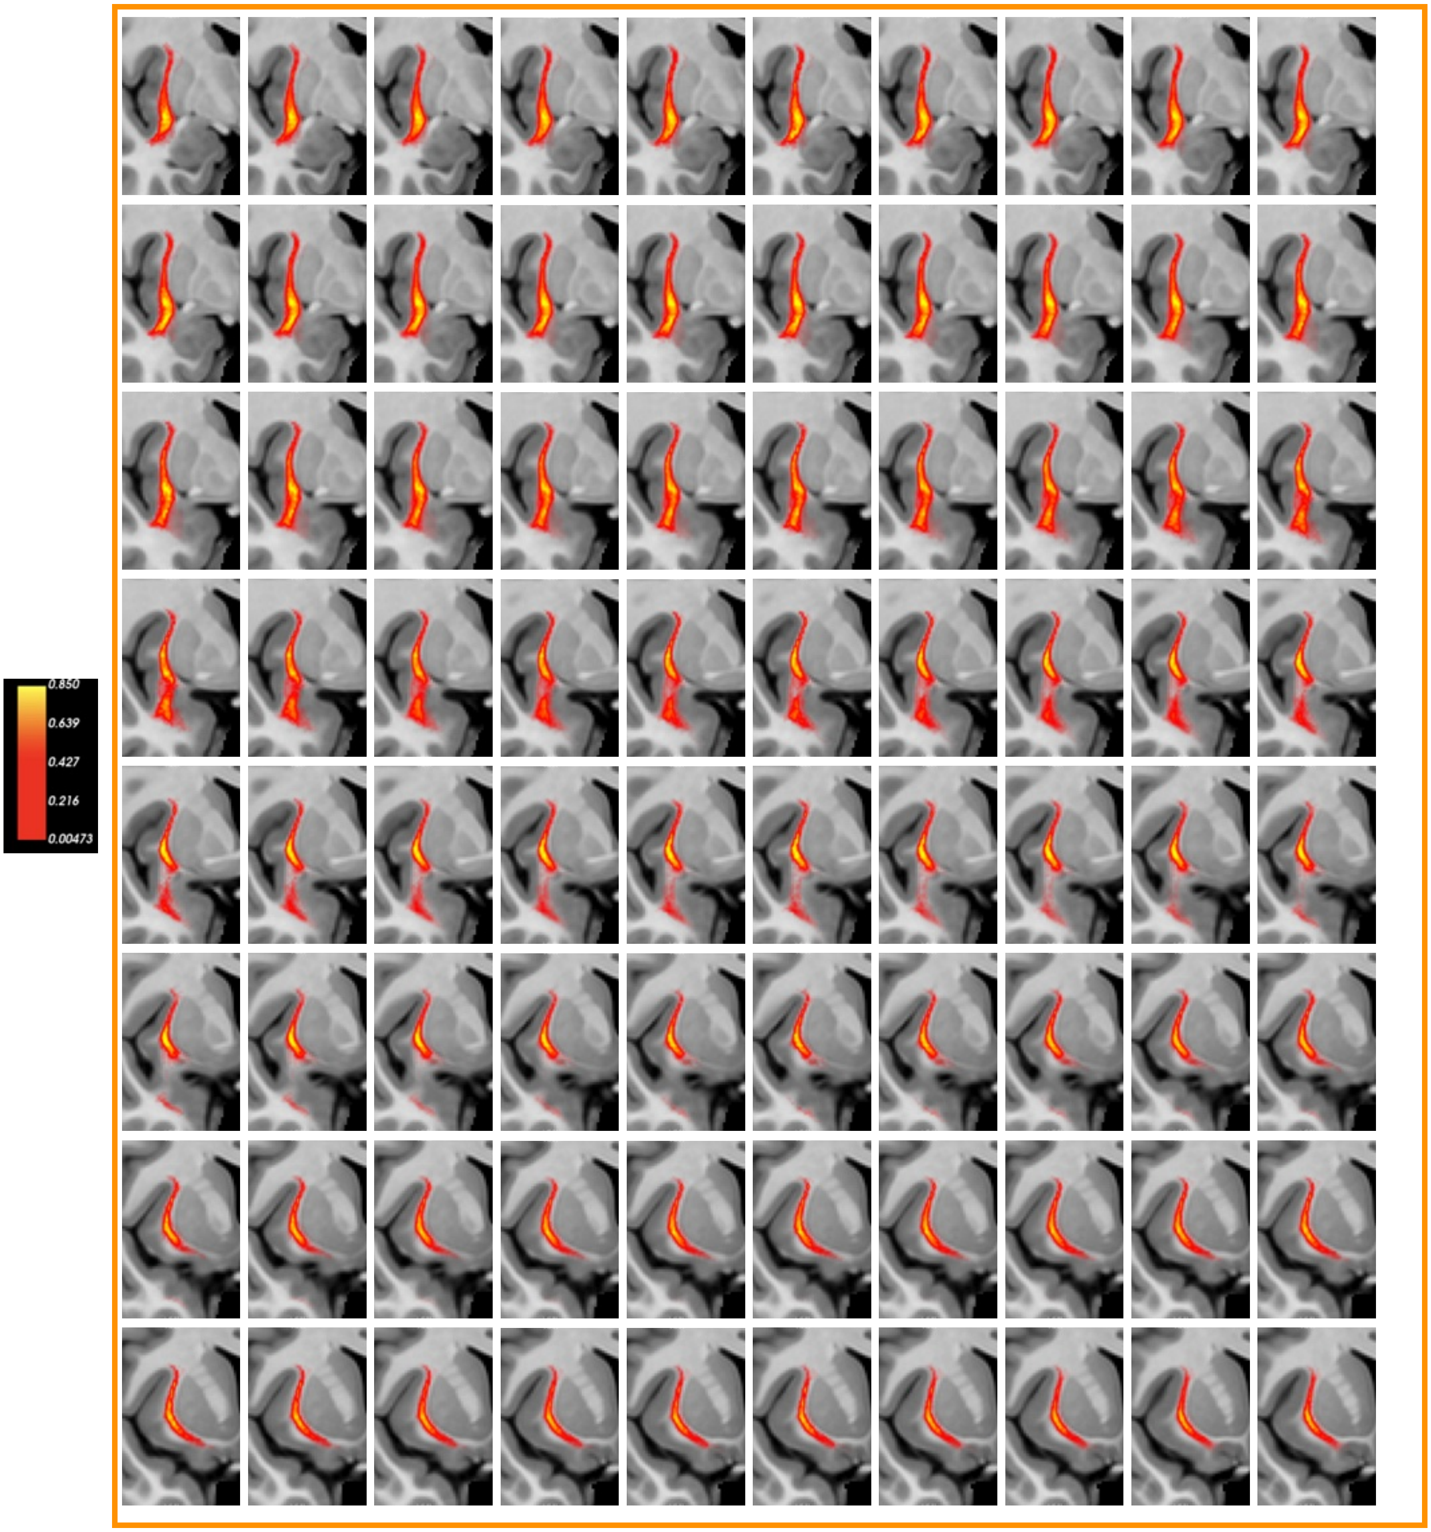


Supplementary Figure 3.2: Coronal slices of the claustrum probabilistic atlas in MNI space, for the right hemisphere (slice numbers: 150 to 229).

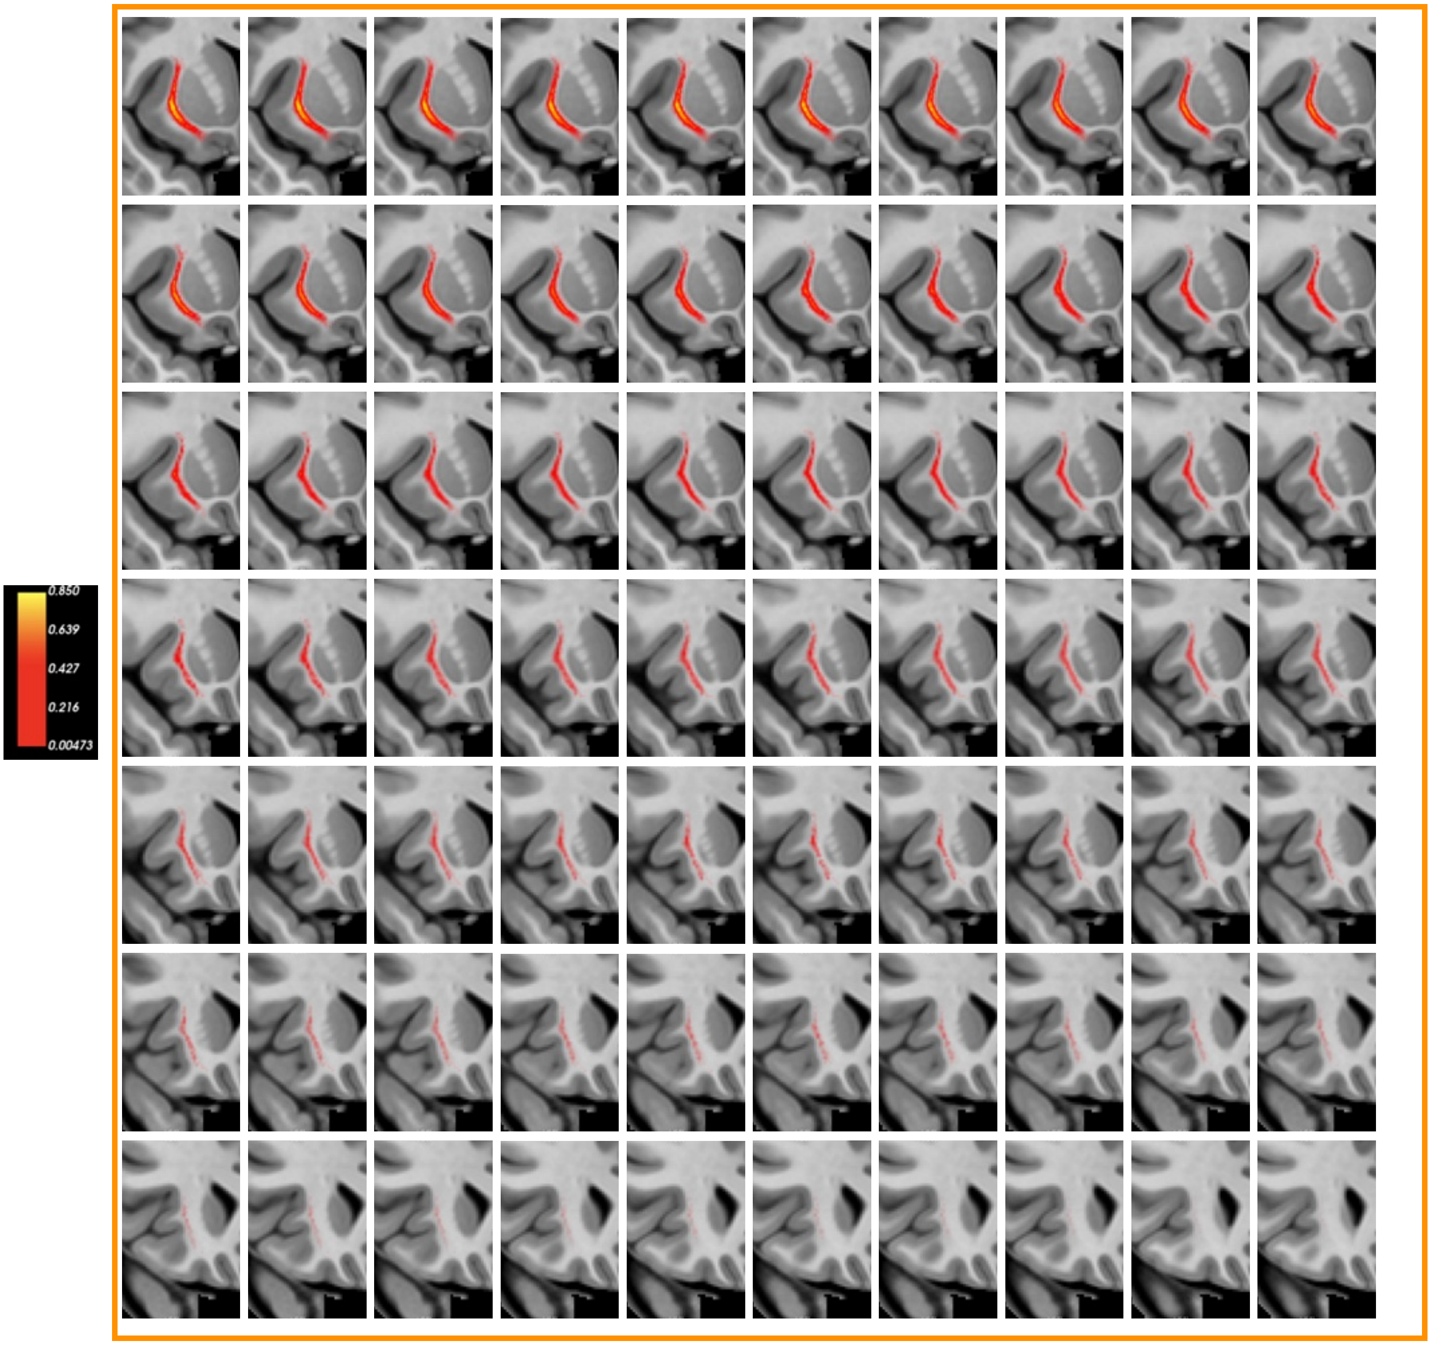


Supplementary Figure 3.3: Coronal slices of the claustrum probabilistic atlas in MNI space, for the right hemisphere (slice numbers: 230 to 299).

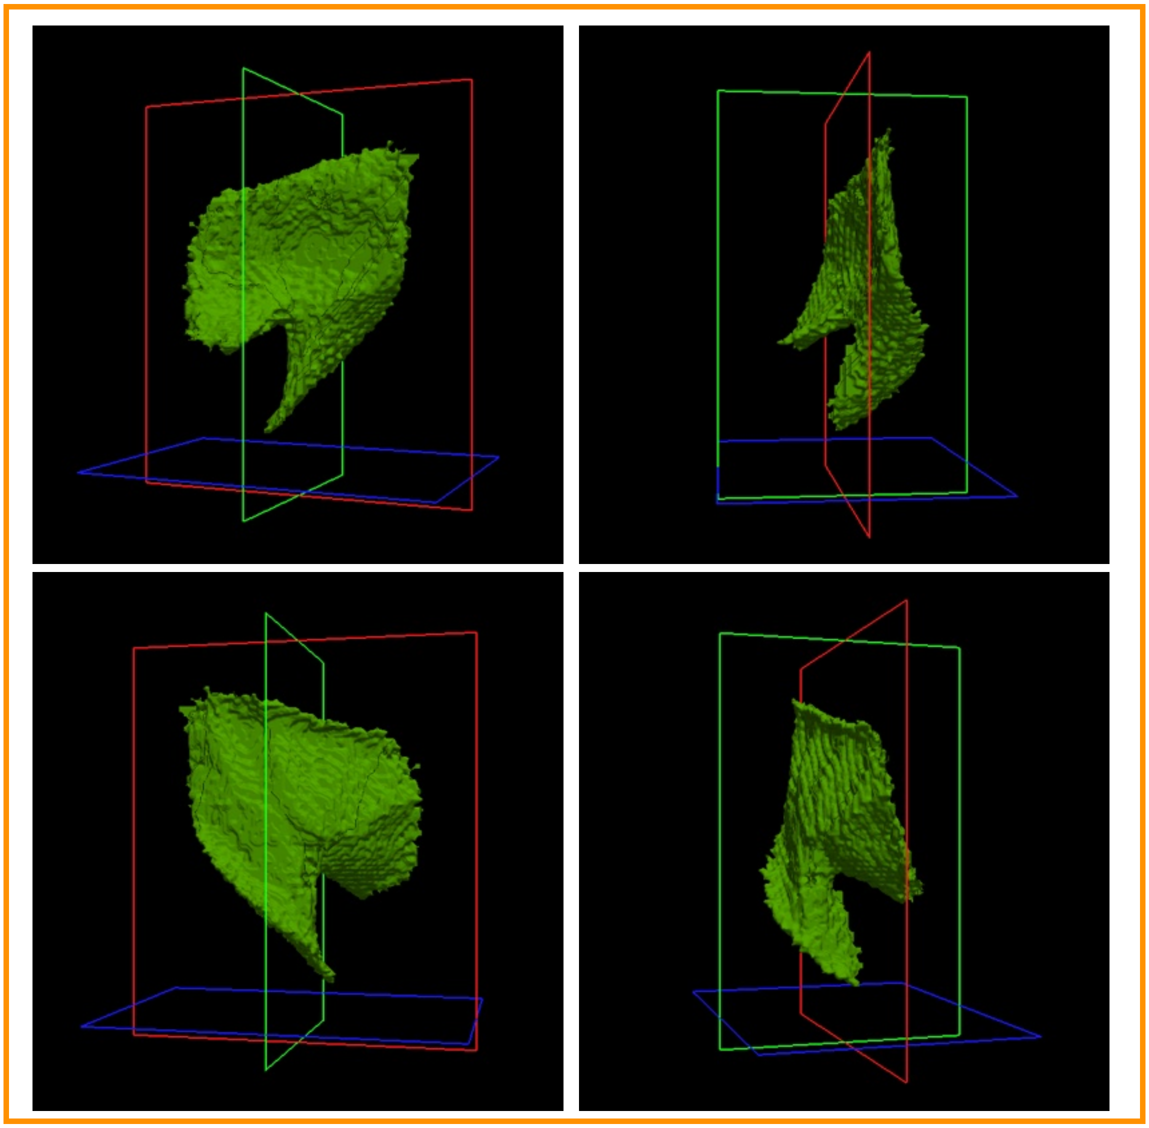

Supplementary Figure 3.4: 3D rendering of the claustrum probabilistic atlas in MNI space for the right hemisphere, thresholded at 0.05.

### Supplementary Section 4: Training and validation curves

Supplementary Fig. 4.1 and Supplementary Fig. 4.2 show the Dice loss and Dice score across epochs for each of the six models trained during 6-fold cross-validation (CV). The Dice loss was optimized during training, on synthetic intensity images, across all ROI structures. The validation Dice score was computed only for claustrum on real validation intensity images, and used to select the best epoch for each model. The Dice score for claustrum computed on the real intensity images corresponding to the training labels is also reported for reference. However, these real images were not used during training, as the models were trained exclusively on synthetic intensity images.

Based on the validation Dice scores for the claustrum, the best performing models are the CV folds 2 and 5 (max Dice = 0.680), while the worst is the CV fold 4 (max Dice = 0.605).

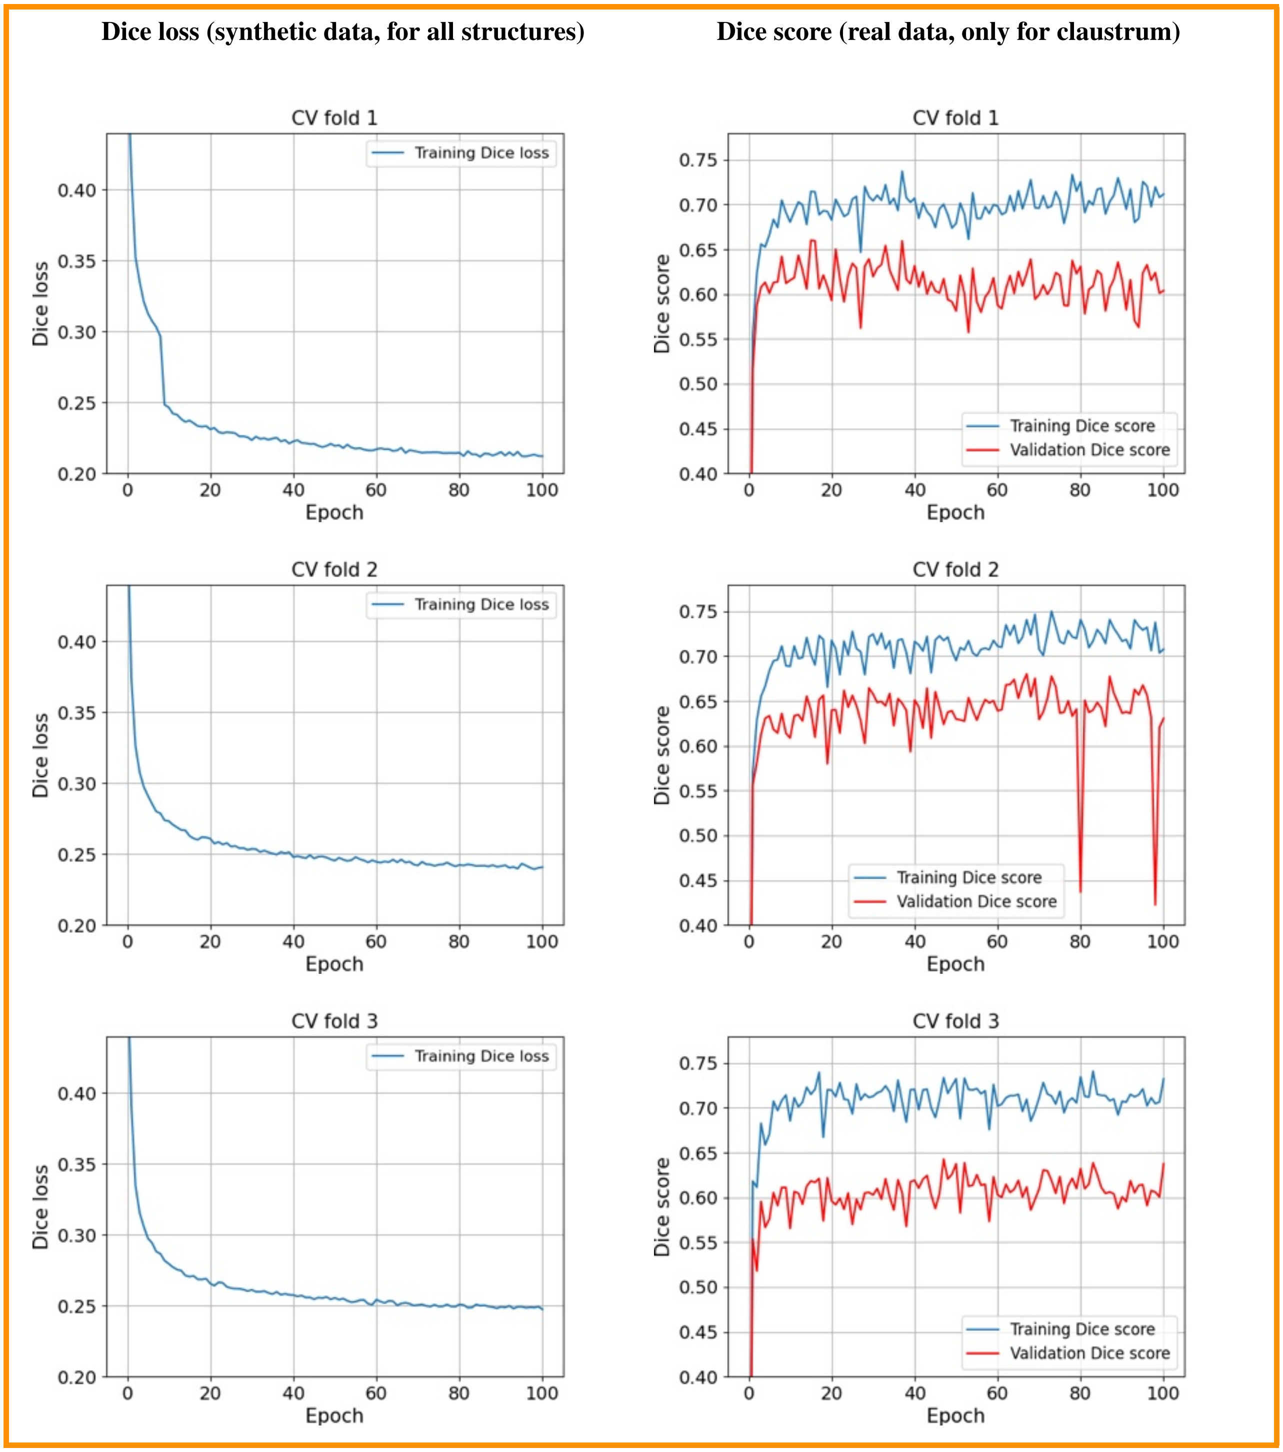


Supplementary Figure 4.1: Training and validation curves for the models in CV folds 1, 2, 3. Left: Training Dice loss, computed on synthetic intensity images, using all structures in the ROI. Right: Training and validation Dice score for claustrum, computed on real intensity images.

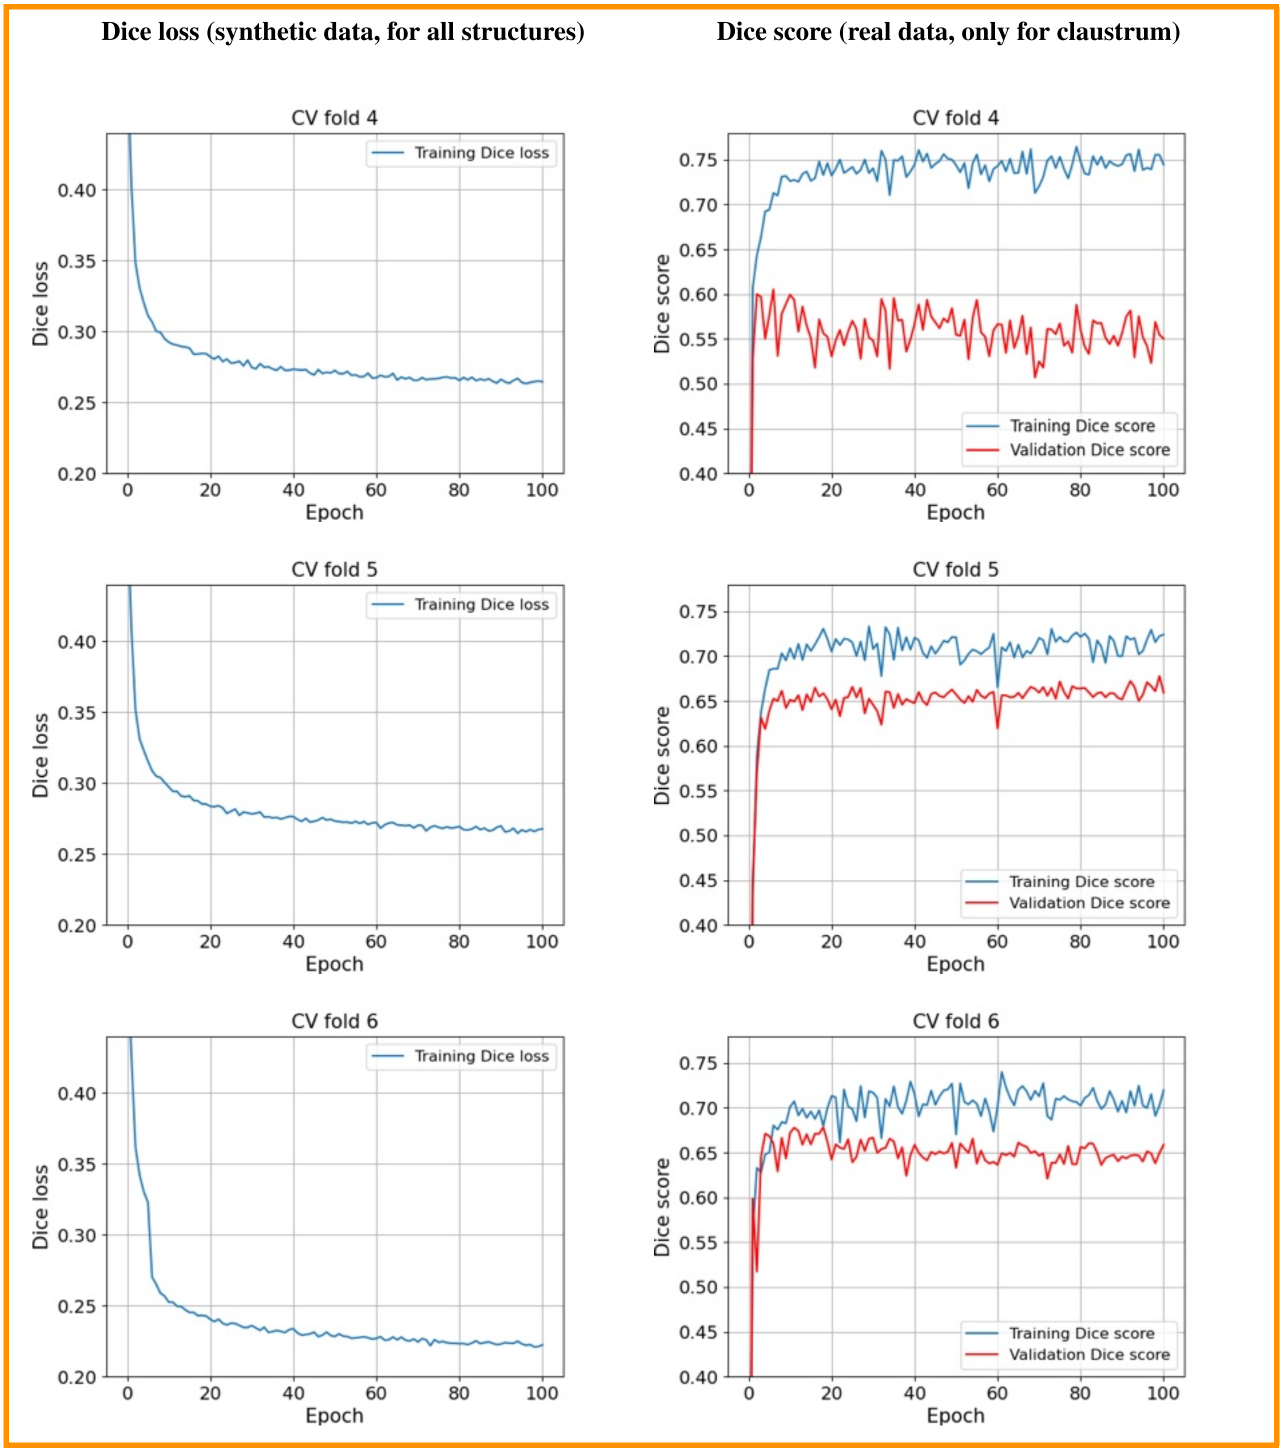


Supplementary Figure 4.2: Training and validation curves for the models in CV folds 4, 5, 6. Left: Training Dice loss, computed on synthetic intensity images, using all structures in the ROI. Right: Training and validation Dice score for claustrum, computed on real intensity images.

### Supplementary Section 5: Assessing the impact of including one *in vivo* case in the training set

During training, whether a case is *in vivo* or *ex vivo* has no impact on the generated intensities, as we synthesize random contrast in all instances. The only potential effect of including the *in vivo* case during training lies in its native label resolution (0.25 mm, compared to 0.10–0.15 mm for the other ones), which is however mitigated by aggressive augmentations and downsampling performed on the labels at training time. To evaluate the effect of incorporating a single *in vivo* case into our high-resolution dataset, we compared CV performance with and without its inclusion. We performed 5-fold CV using only the 16 *ex vivo* hemispheres, yielding a Dice score of 0.633 ± 0.060. This is comparable to the 0.632 ± 0.061 obtained when including the *in vivo* case (see Table 2), indicating that its inclusion does not influence performance. Nevertheless, we retained this case in the study to maximize the number of available training samples.

### Supplementary Section 6: Assessing the impact of training on labels from rater 1 vs. the rater 2

As detailed in Sec. 3.1, rater 2 independently re-labeled the seven hemispheres previously labeled by rater 1 (cases 4, 13, 14, 15, 16) to assess inter-rater variability. Since labeling was performed sequentially, the annotations from the two raters were not merged into final training labels, as is typically done. Instead, for these seven commonly labeled hemispheres, we used the annotations from rater 1 as training labels and annotations from rater 2 only to compute Dice score vs. rater 1. To evaluate the impact of this design choice on segmentation performance, we trained two additional models - one per rater - using only the seven commonly labeled hemispheres, and tested them on the remaining 11 cases. Validation curves in Supplementary Fig. 6.1 indicate comparable performance, with peak Dice scores of 0.621 (epoch 34, rater 1) and 0.620 (epoch 6, rater 2), suggesting that the choice of rater did not introduce bias.

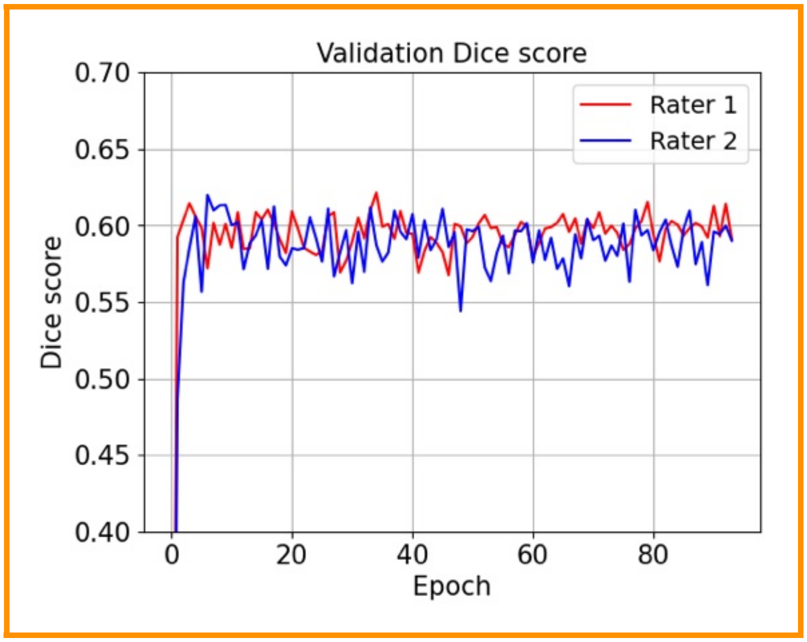


Supplementary Figure 6.1: Validation Dice scores for claustrum across epochs for models trained on cases 4, 13, 14, 15, and 16. One model was trained using labels from rater 1, while the other model used labeled from rater 2. The validation set consists of the remaining 11 hemispheres.

### Supplementary Section 7: 3D rendering of *in vivo* claustrum segmentations

Supplementary Fig. 7.1, Supplementary Fig. 7.2, and Supplementary Fig. 7.3 show 3D renderings of claustrum segmentations from representative subjects in the IXI, Miriad, and FSM datasets, respectively.

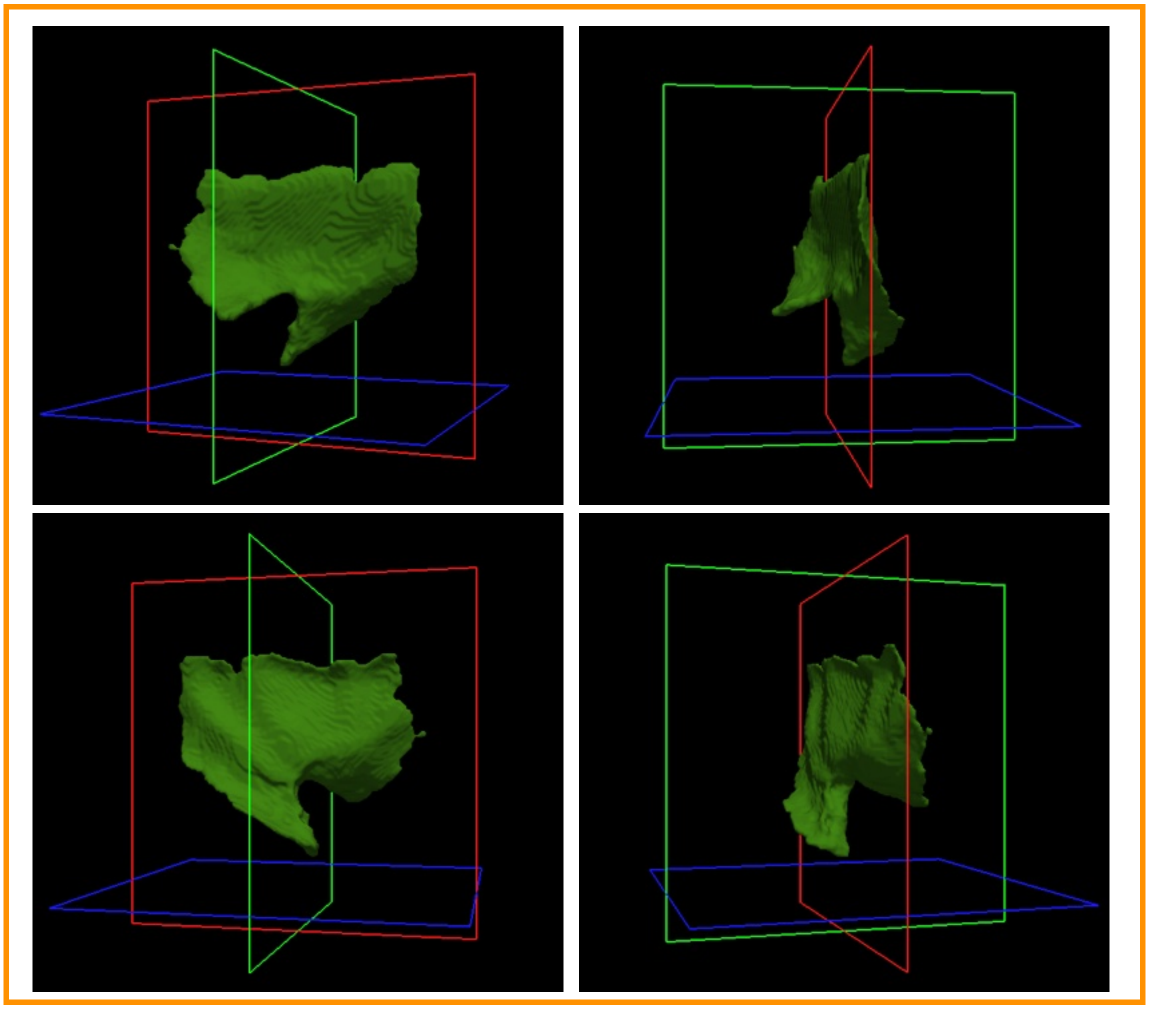

Supplementary Figure 7.1: 3D rendering of claustrum segmentation on the right hemisphere for a subject from the IXI dataset (ID: 150). The QC score for this segmentation is 0.571. The subject was selected for its representative score.

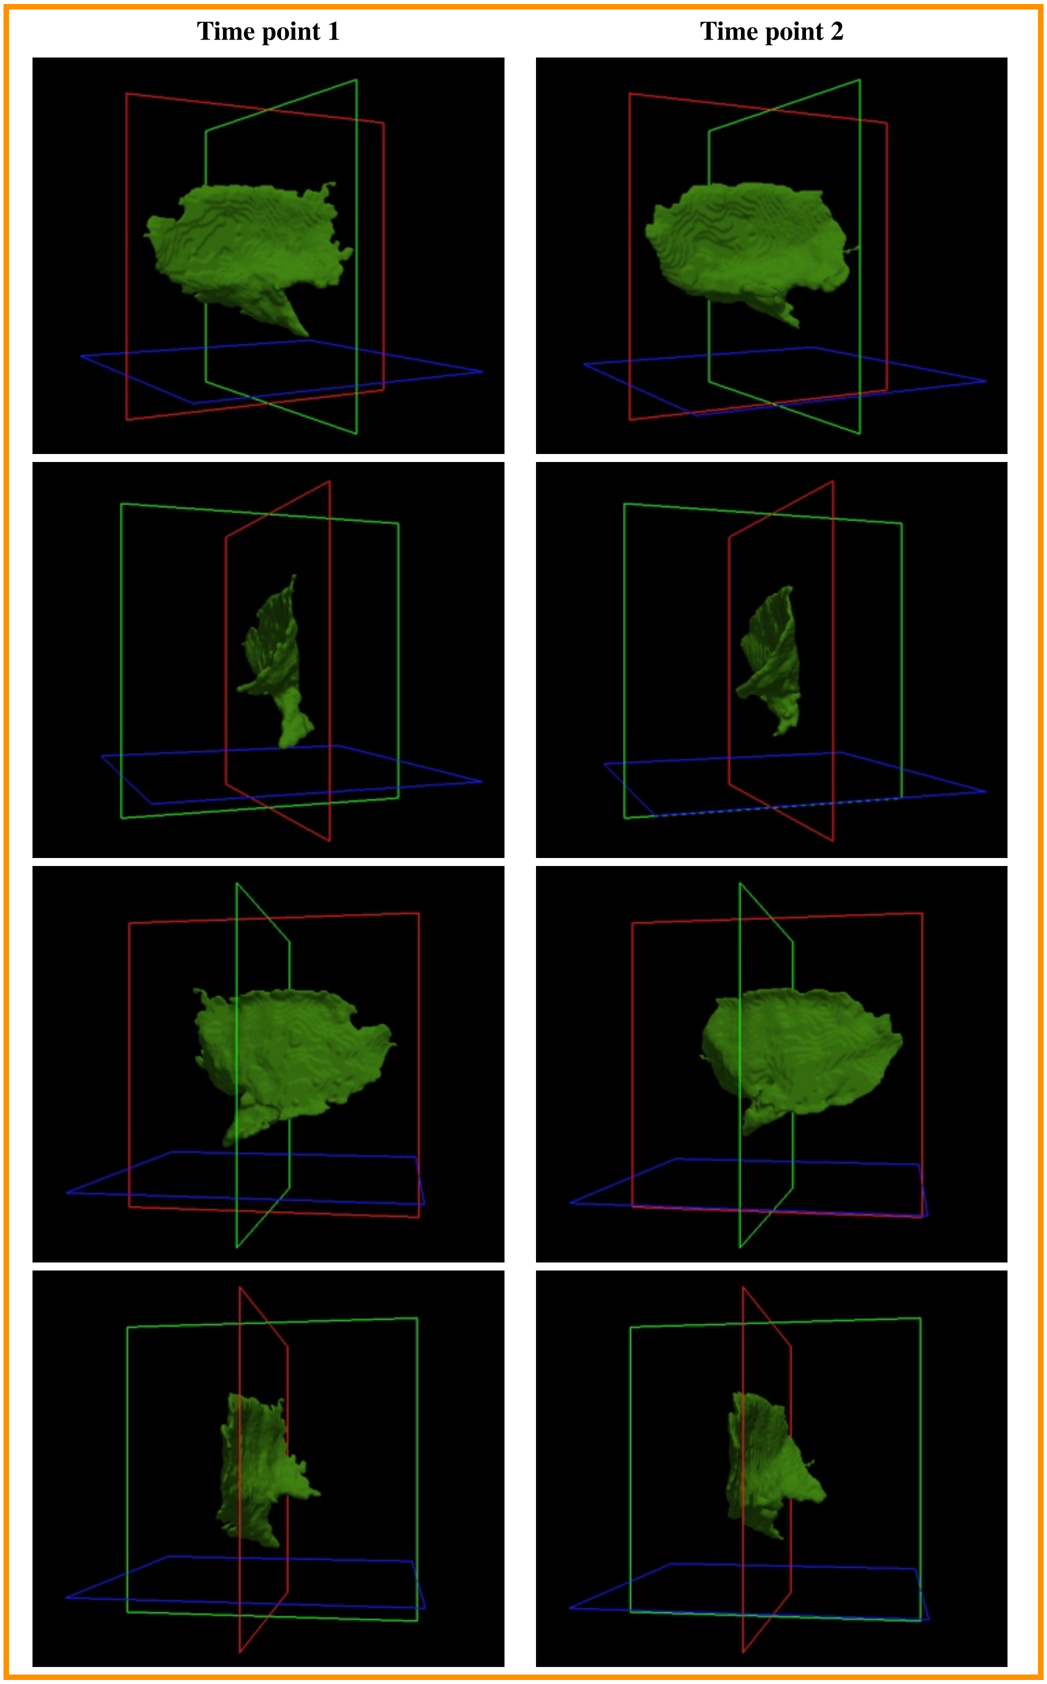


Supplementary Figure 7.2: 3D rendering of left-hemisphere claustrum segmentation in a healthy subject from the Miriad dataset (ID: 247). Left: Segmentation from the first time point scan. Right: Segmentation from the second time point scan. The test-retest Dice score for this segmentation is 0.793. This subject was selected for its representative score.

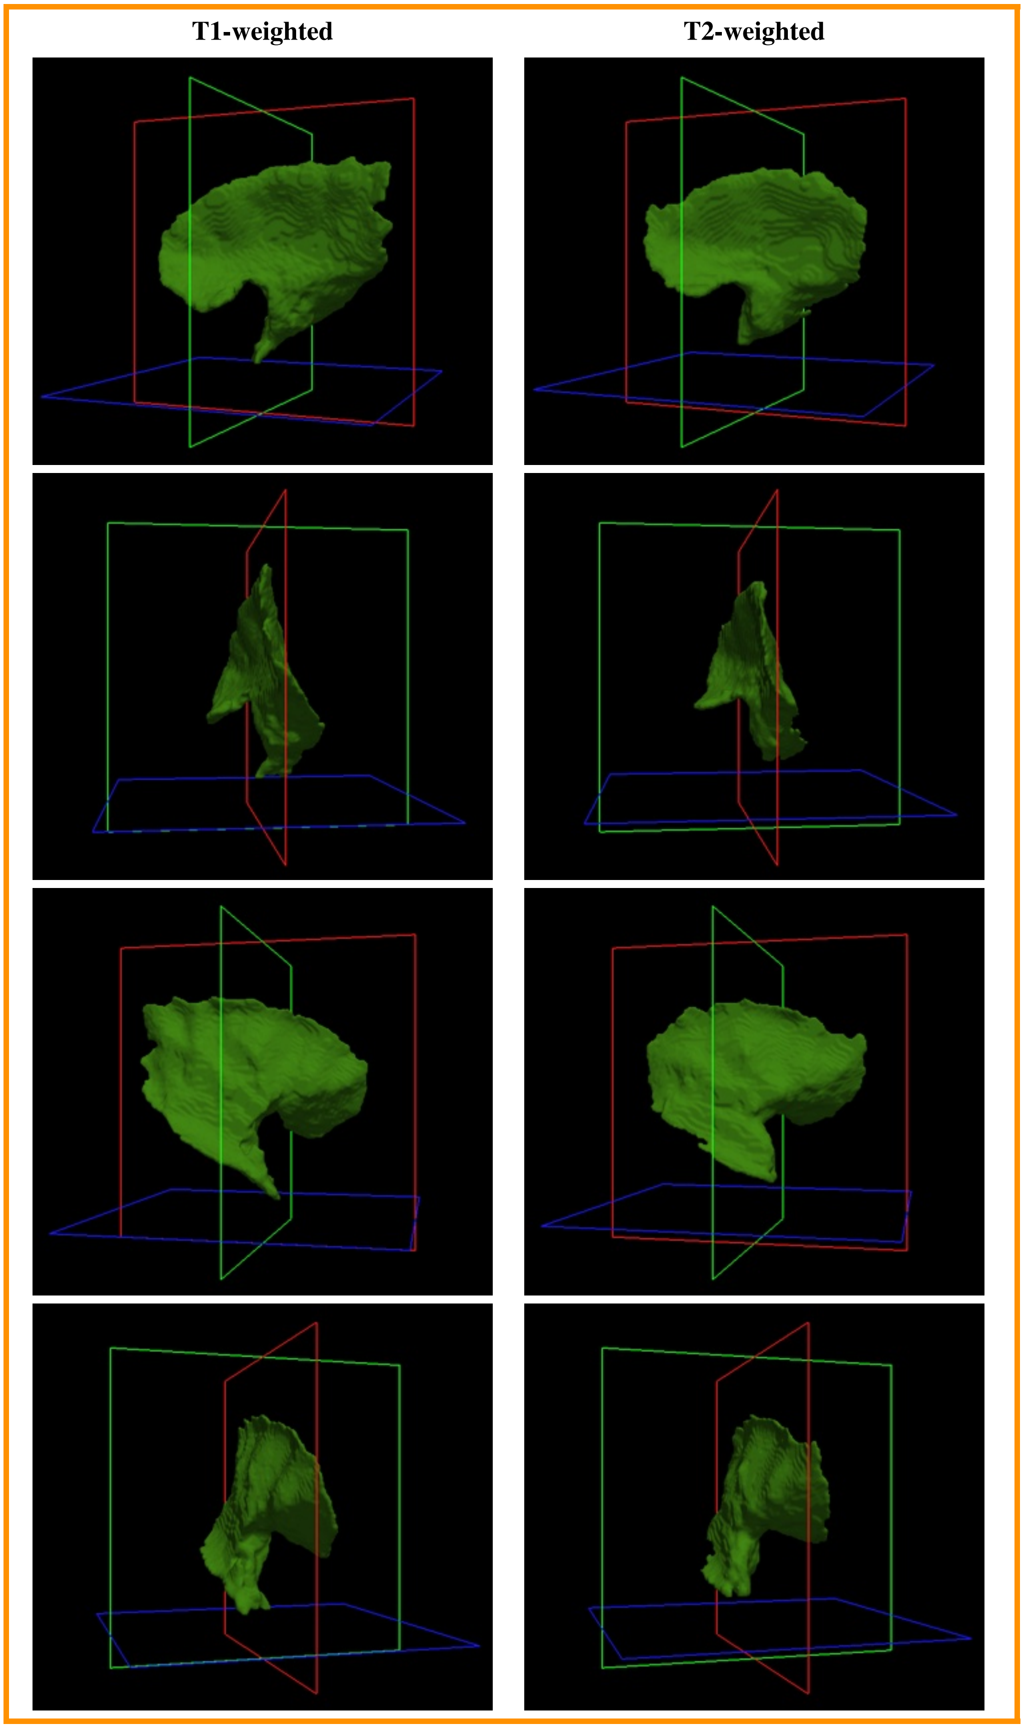


Supplementary Figure 7.3: 3D rendering of claustrum segmentation on the right hemisphere for a subject from the FSM dataset (ID: 002). Left: Segmentation from the T1-weighted image. Right: Segmentation from the T2-weighted image. The Dice score between T1-weighted and T2-weighted segmentations is 0.724. This subject was selected for its representative Dice score.

**Supplementary Section 8: Detecting age effects in claustrum volumes**

The dataset of high-resolution hemispheres used for training has an average age of 61.94 ± 13.66 years, which may hamper the model generalizability to younger subjects. This limitation, typical of *ex vivo* datasets, is somewhat mitigated by the extensive augmentation and image synthesis performed by SynthSeg, which expose the model to significant variability. To investigate this, we analyzed claustrum volumes against age in the IXI dataset, which covers the entire adult lifespan (Supplementary Fig. 8.1). The analysis reveals a decreasing trend of volume with age, showing that the model is able to detect, at least partially, age-related changes in the volume of the claustrum.

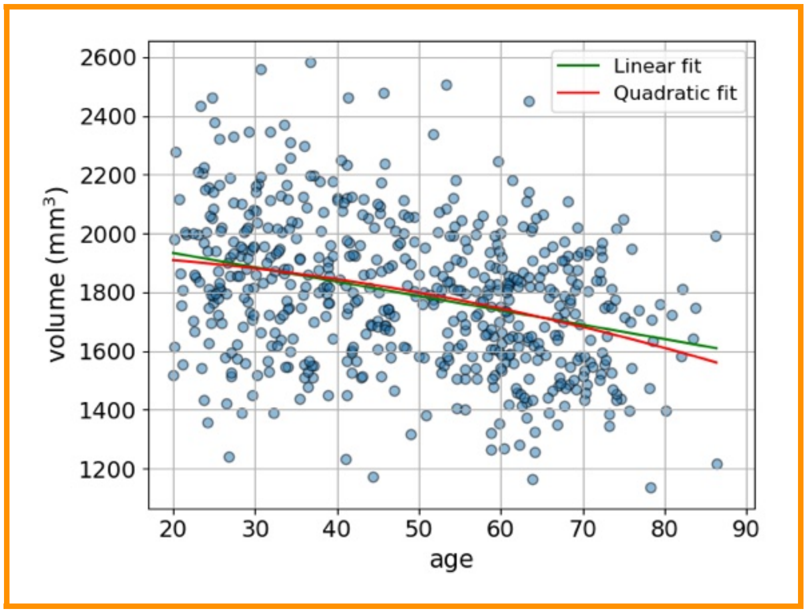


Supplementary Figure 8.1: Claustrum hemispheric volume against age on the IXI dataset. We computed a linear and quadratic fit to the data, showing a decreasing trend of volume with age.
